# Supplementary material for: Citadel: Protecting Data Privacy and Model Confidentiality for Collaborative Learning with SGX
Source: arXiv:2105.01281 source file (2021-11-08)
Supplement: Supplementary file 1 [file 09appendix.tex]

%!TEX root = main.tex
\appendix
%Appendix A
\section{dACIQ: Analytical Model of Gradient Quantization}
